# Supplementary material for: Probing quantum geometric nonlinear magnetization via second-harmonic magneto-optical Kerr effect
Source: arXiv:2602.03636 source file (2026-02-03)
Supplement: Supplementary file 1 [file Supp.pdf]

# Supplemental Material for "Probing quantum geometric nonlinear magnetization via second-harmonic magneto-optical Kerr effect"

Xuan Qian,[1,2,*] Xiao-Bin Qiang,[3,*] Wenkai Zhu,[1,2,*] Yuqing Huang,[1,2]
Yiyuan Chen,[3,4] Hai-Zhou Lu,[3,4,†] Yang Ji,[5,‡] and Kaiyou Wang[1,2,§]

[1] *State Key Laboratory of Semiconductor Physics and Chip Technologies, Institute of Semiconductors, Chinese Academy of Sciences, Beijing 100083, China*
[2] *College of Materials Science and Optic-Electronic Technology, University of Chinese Academy of Sciences, Beijing 100049, China*
[3] *State Key Laboratory of Quantum Functional Materials, Department of Physics, and Guangdong Basic Research Center of Excellence for Quantum Science, Southern University of Science and Technology (SUSTech), Shenzhen 518055, China*
[4] *Quantum Science Center of Guangdong-Hong Kong-Macao Greater Bay Area (Guangdong), Shenzhen 518045, China*
[5] *School of Physics, Zhejiang University, Hangzhou, China*

(Dated: February 3, 2026)

In this Supplemental Material, we present experimental and theoretical details, which includes Refs. [1–14].

## CONTENTS

SI. Symmetry Analysis of Magnetization Coefficients S2

SII. Device Fabrication S3

SIII. Polarization-Dependent Raman Measurement S3

SIV. Electrical Transport Measurements S4
- A. I-V Curves at Different Temperatures S4
- B. Nonlinear Hall Effect at Different Temperatures S6

SV. Second-Harmonic Magneto-Optical Kerr Effect Measurements S7

SVI. Experimental Data in Graphene Control Device S8

SVII. Laser Intensity Dependence of the SMOKE S10

SVIII. Theory of Nonlinear Magnetization S10
- A. Boltzmann Kinetics for Non-equilibrium Distribution Function S10
- B. Calculation of Nonlinear Spin Magnetization Coefficient S11
- C. Calculation of Nonlinear Orbital Magnetization Coefficient S12

SIX. Estimation of Scattering Time S14

References S14

* These authors contributed equally to this work.
† luhz@sustech.edu.cn
‡ jiyang2024@zju.edu.cn
§ kywang@semi.ac.cn

## SI. SYMMETRY ANALYSIS OF MAGNETIZATION COEFFICIENTS

The generation of magnetization by an applied electric field characterized by the magnetization coefficient $\boldsymbol{\alpha}$ as

$$\delta M_i = \alpha_{ij} E_j + \alpha_{ijk} E_j E_k, \tag{S1}$$

where $i, j$ are spatial indices and the Einstein summation is implied. The coefficient $\alpha_{ij}$ characterizes linear response, while $\alpha_{ijk}$ characterizes nonlinear response.

For systems with inversion symmetry $\mathcal{P}$, the linear response is strictly forbidden because the magnetization vector is an axial vector, which remains invariant under inversion. For the time-reversal symmetry $\mathcal{T}$, the restriction to the response coefficients depends on the parity of the powers of the relaxation time $\tau$. The detailed forms of $\boldsymbol{\alpha}$ constrained by symmetry are presented in Table S1.

TABLE S1. Constraints on magnetization coefficient from $\mathcal{P}$, $\mathcal{T}$ and $\mathcal{PT}$ symmetries. ✓(✗) means that the symmetry operation is allowed (forbidden), and $n$ represents the integer.

| | $\mathcal{P}$ | $\mathcal{T}$ | $\mathcal{PT}$ |
|---|---|---|---|
| $\alpha_{ij} \propto \tau^{2n}$ | ✗ | ✗ | ✓ |
| $\alpha_{ij} \propto \tau^{2n+1}$ | ✗ | ✓ | ✗ |
| $\alpha_{ijk} \propto \tau^{2n}$ | ✓ | ✗ | ✗ |
| $\alpha_{ijk} \propto \tau^{2n+1}$ | ✓ | ✓ | ✓ |

For system with time-reversal symmetry, i.e., non-magnetic system, all intrinsic contributions $\propto \tau^0$ vanishes identically. This is the case that we shall discuss in this article. Additionally, the nonlinear magnetization coefficient $\alpha_{ijk}$ must preserves the point group symmetry:

$$\alpha_{i'j'k'} = \det(\mathcal{O}) \mathcal{O}_{i'i} \mathcal{O}_{j'j} \mathcal{O}_{k'k} \alpha_{ijk}, \tag{S2}$$

where $\mathcal{O}$ is representation matrix for the point group operation in Cartesian coordinate. Assuming the polar configuration, i.e., the electric field applying along the $\hat{x}$ or $\hat{y}$ direction, the point group symmetry constraints are listed in Table S2.

TABLE S2. Constraints on nonlinear magnetization coefficient from point group symmetries. ✓(✗) means that the symmetry operation is allowed (forbidden). $\mathcal{C}_i^n$ denotes the $n$-fold rotation ($n = 2, 3, 4, 6$) with respect to the Cartesian axis along the $i$-direction, $\mathcal{M}_i$ represents a mirror with respect to the plane normal to the $i$-direction, and $\mathcal{S}_i^n = \mathcal{C}_i^n \mathcal{M}_i$ represents improper rotation.

| | $\mathcal{C}_z^2$ | $\mathcal{C}_z^{3,4,6}$ | $\mathcal{C}_x^{2,4,6}(\mathcal{C}_y^{2,4,6})$ | $\mathcal{C}_x^3$ | $\mathcal{C}_y^3$ | $\mathcal{S}_z^{4,6}$ | $\mathcal{S}_x^4(\mathcal{S}_y^4)$ | $\mathcal{S}_x^6$ | $\mathcal{S}_y^6$ | $\mathcal{M}_z$ | $\mathcal{M}_x(\mathcal{M}_y)$ |
|---|---|---|---|---|---|---|---|---|---|---|---|
| $\alpha_{zxx}$ | ✓ | ✓ | ✗ | ✗ | ✓ | ✓ | ✗ | ✗ | ✓ | ✓ | ✗ |
| $\alpha_{zyy}$ | ✓ | ✓ | ✗ | ✓ | ✗ | ✓ | ✗ | ✓ | ✗ | ✓ | ✗ |

## SII. DEVICE FABRICATION

High-quality Td-phase $WTe_2$ and hexagonal boron nitride (h-BN) are purchased from HQ Graphene Company. Van der Waals heterostructures were assembled via polydimethylsiloxane (PDMS)-assisted dry transfer technique. $WTe_2$ flakes were first mechanically exfoliated onto a PDMS stamp. Flakes of desired thickness and morphology were identified under an optical microscope (Olympus) and transferred onto a target substrate using a home-built three-dimensional hydraulic micro-manipulation system. Prior to the transfer, Ti(5 nm)/Au(20 nm) electrodes were pre-patterned on a Si/$SiO_2$ substrate via standard electron-beam lithography, magnetron sputtering and lift-off processes. The final stack, from bottom to top, consists of the Si/$SiO_2$ substrate with pre-patterned electrodes, a $WTe_2$ flake, and a protective h-BN capping layer. The device was subsequently annealed at 120°C for 10 minutes to improve the electrical contact. Control devices were fabricated following an identical process. All fabrication steps were carried out in a nitrogen-filled glove box with oxygen and moisture levels maintained at less than 1 ppm. A schematic of the device is shown in Fig. S1(a) along with its optical micrograph [Fig. S1(b)]. The layer thicknesses of $WTe_2$ and h-BN are 7 nm and 16 nm, respectively. It is confirmed by atomic force microscope, as illustrated in Figs. S1(c) and (d).

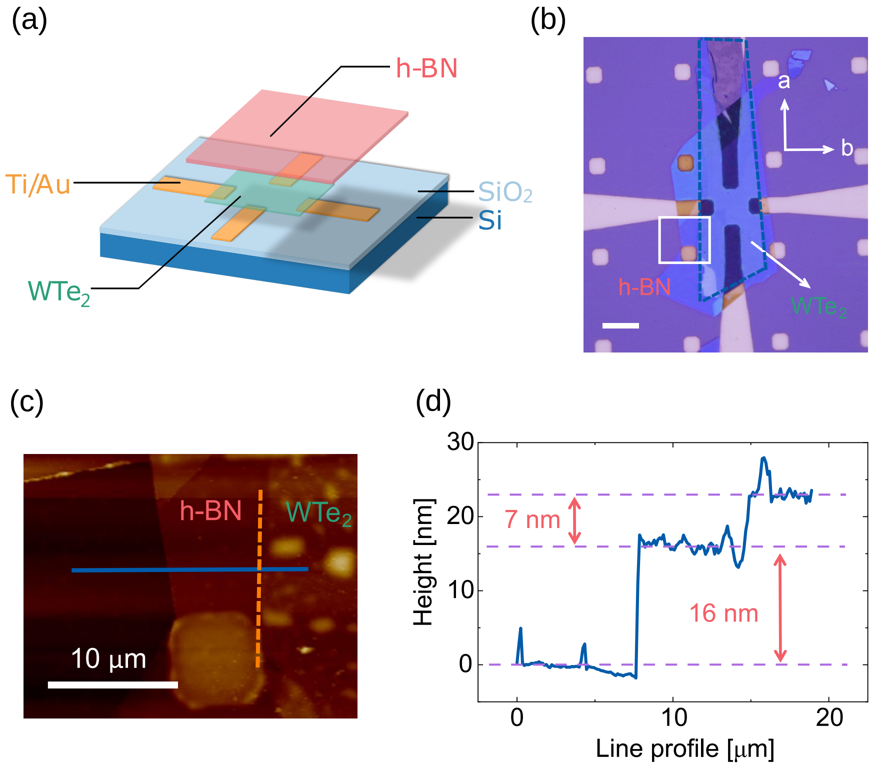


FIG. S1. Device fabrication and characterization. (a) Schematic of the device. (b) An optical image of the device. The electrodes are set up to allow the application of current along the $a$ and $b$ axis of $WTe_2$. The $WTe_2$ and h-BN flakes are clearly labeled. The scale bar is 10 $\mu$m. (c) The atomic force microscope image of the device. The scanning range is shown as the white square area in (b). (d) The line profile shows the thickness of the $WTe_2$ and h-BN are 7 nm and 16 nm, respectively.

## SIII. POLARIZATION-DEPENDENT RAMAN MEASUREMENT

Polarization-dependent Raman measurements were performed at room temperature using a commercial micro-Raman system (Horiba Jobin Yvon HR800) in a backscattering configuration. A 50× objective lens, an 1800 grooves per mm grating, and an integration time of 30 seconds were used to obtain high-resolution spectra. The incident laser power was maintained below 320 $\mu$W to avoid sample damage. To study the polarization dependence, the incident polarization was set by a fixed polarizer and rotated by a half-wave plate. The polarization of the scattered light was analyzed by a second polarizer placed before the spectrometer entrance. Figure 1(b) presents the corresponding contour plot of the integrated Raman intensity. The 212 $cm^{-1}$ peak shows a clear intensity minimum when the laser polarization aligns with the sample edge [Fig. 1(c)]. This characteristic polarization dependence, in agreement with

previous work [1], was used to confirm the $a$ axis orientation.

## SIV. ELECTRICAL TRANSPORT MEASUREMENTS

Electrical transport measurements were carried out in a Janis vibration-isolated microscopy cryostat system, featuring an operational temperature range from 6.5 K to 325 K. First- and second-harmonic signals were acquired using a Stanford Research Systems Model SR830 lock-in amplifier, operating at a frequency of 117.77 Hz. The integration time and filter roll-off were set at 3 seconds and 24 dB per octave, respectively. The phase of the first-harmonic signal was set to 0°, while that of the second-harmonic signal was set to 90°, corresponding to the expected values for first- and second-order responses, respectively.

As shown in Fig. S2, the AC source was generated by the SR830 lock-in amplifier's internal oscillator, offering an adjustable amplitude range from 4 mV to 5 V with 2 mV resolution. During the experiments, the SR830 voltage source was connected in series with a protective resistor ($R_p$=10 kΩ), while its negative terminal was directly grounded. For current along the $a$ axis, both transverse and longitudinal first- and second-harmonic signals were systematically measured. The same measurement protocol was then implemented for current along the $b$ axis, with harmonic components in both orthogonal directions quantified through phase-sensitive detection.

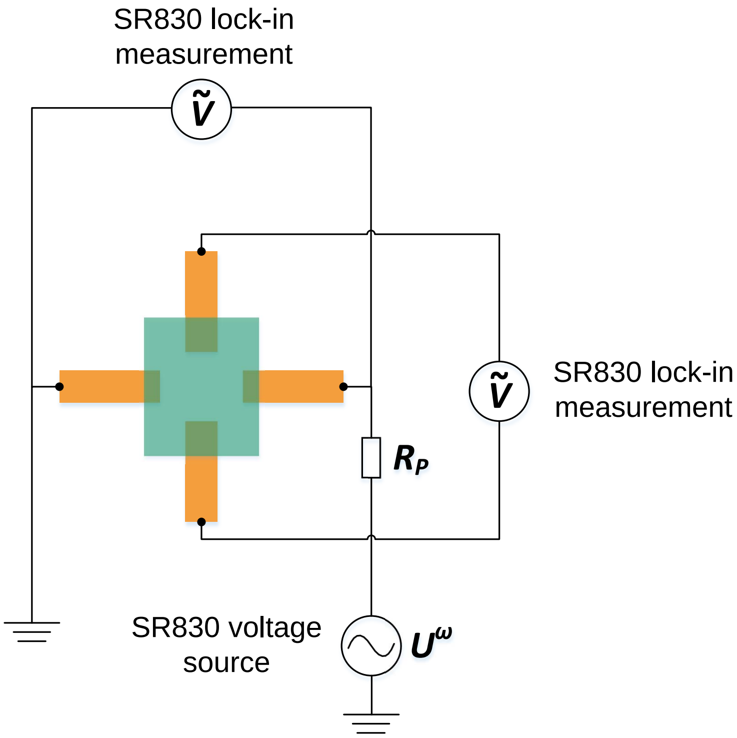


FIG. S2. Schematic structure of the circuit for electrical transport measurements. The schematic shows the setup for measuring transverse and longitudinal first- and second-harmonic signals in $WTe_2$. A SR830 lock-in amplifier supplies an AC voltage through a protective resistor ($R_p$=10 kΩ), with its negative terminal grounded. Current is applied along the $a$ and $b$ crystallographic axes. First- and second-harmonic phases are set to 0° and 90°, respectively.

### A. I-V Curves at Different Temperatures

To determine the current passing through the sample at various temperatures and the corresponding voltage across its terminals, we measured the current–voltage (I–V) curves for currents flowing along the $a$ axis and $b$ axis directions at different temperatures. The results are plotted in Figs. S3(a) and (c), where the I-V curves demonstrate excellent linearity within the temperature range from 8 K to 200 K. Figs. S3(b) and (d) illustrate the temperature dependence

of the resistance along the crystal $a$ axis and $b$ axis, respectively. They increase nearly linearly with temperature and both display characteristic metallic behavior.

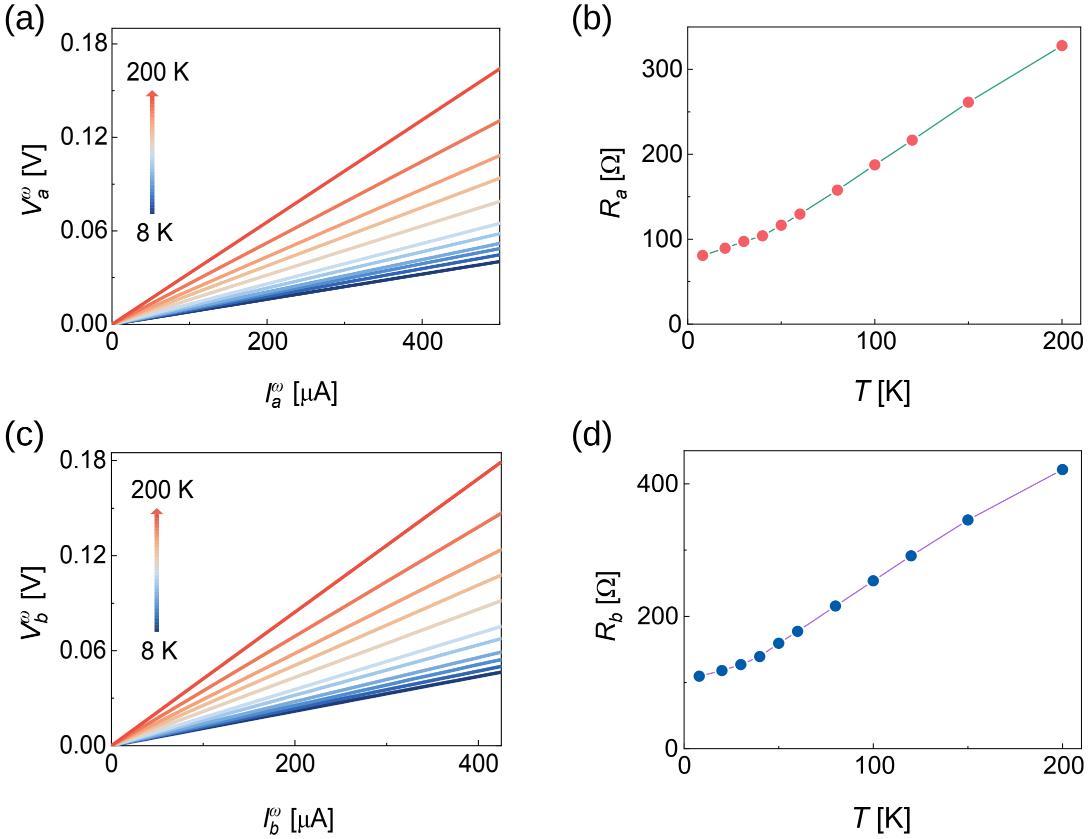


FIG. S3. I-V characteristics at different temperatures. (a,b) The I-V characteristics and the corresponding temperature-dependent resistance for current applied along the crystal $a$ axis (in the order 8, 20, 30, 40, 50, 60, 80, 100, 120, 150 and 200 K). (c,d) The I-V characteristics and the corresponding temperature-dependent resistance for current applied along the crystal $b$ axis, measured over an identical temperature series.

### B. Nonlinear Hall Effect at Different Temperatures

The temperature evolution of the nonlinear Hall effect in $WTe_2$ device is summarized in Fig. S4. The transverse voltage exhibits a clear quadratic dependence when the current is applied along the $a$ axis, as shown in Fig. S4(a), where all data are well fitted with quadratic functions (solid lines). Notably, the nonlinear Hall signal becomes nearly undetectable above 150 K. Fig. S4(b) shows the linear scaling relation between the nonlinear Hall response and the longitudinal conductivity. The conductivity $\sigma$ is derived from the resistance $R$ using the geometric relation $\sigma = L/(WtR)$, where $L = 15\ \mu m$ , $W = 5\ \mu m$, and $t = 7\ nm$ are the channel length, width, and material thickness, respectively.

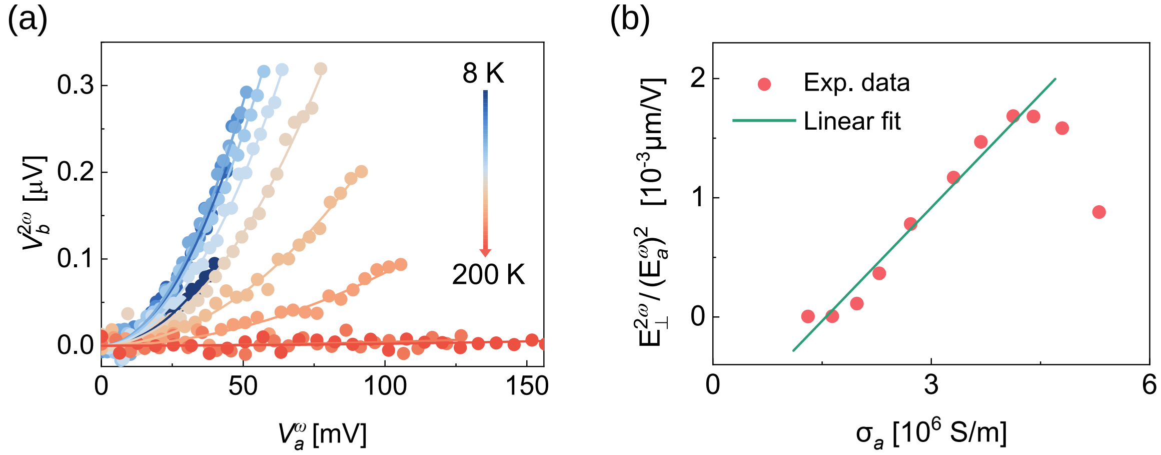


FIG. S4. Temperature-dependent nonlinear Hall response in $WTe_2$. (a) The nonlinear Hall voltage as a function of applied current along the $a$ axis at various temperatures (in the order 8, 20, 30, 40, 50, 60, 80, 100, 120, 150 and 200 K). (b) Scaling behavior between the nonlinear Hall response and longitudinal conductivity for different temperatures from $T = 8$ K to $T = 200$ K.

## SV. SECOND-HARMONIC MAGNETO-OPTICAL KERR EFFECT MEASUREMENTS

Figure S5 shows a detailed schematics of our experimental setup. As in the electrical transport measurements, the device was placed in a Janis vibration-isolated microscopy cryostat system. For polar SMOKE detection, we used a tunable diode laser (Toptica DLC pro 780) at $\lambda$ = 800 nm (1.55 eV), attenuated to a power of about 500 $\mu$W. The beam was incident perpendicular to the sample surface, making the measurement sensitive to out-of-plane magnetic moments. The optical beam was focused onto the sample to a spot size of approximately 3 $\mu$m using a long-working-distance microscope objective with a numerical aperture (NA) of 0.28.

The polarization state of the reflected laser beam was measured using a balanced detection setup. This setup comprised a Wollaston prism, which split the light into two beams polarized linearly and perpendicular to each other, and a balanced detector to measure the intensity difference between these beams. The difference, proportional to the polarization rotation, was initially adjusted to zero by rotating a half-wave plate positioned in front of the Wollaston prism. The signal from the balanced detector was then fed into a lock-in amplifier. The amplifier demodulated the signal at the first- and second-harmonic frequencies of the applied current, extracting the corresponding Kerr rotation components, denoted as the MOKE and SMOKE. The integration time and filter roll-off were set at 3 seconds and 24 dB per octave, respectively.

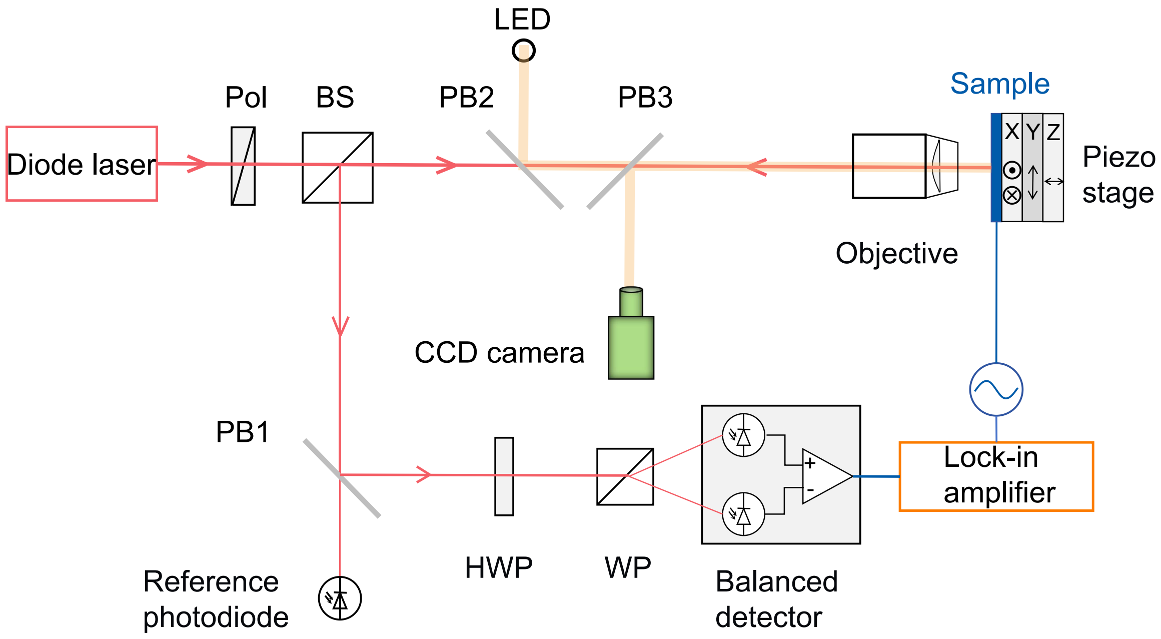


FIG. S5. Schematic drawing of the polar SMOKE measurements. The laser beam sequentially passes through a polarizer (Pol) and a beam splitter (BS) before being focused onto the sample via an objective lens. The reflected light is collimated by the same objective and divided into two beams by a plate beamsplitter (PB1), with one beam directed to a reference photodiode for intensity monitoring. Polarization rotation analysis is performed in a separate detection arm equipped with a half-wave plate (HWP), Wollaston prism (WP), and balanced photodiode detector. The illumination system comprises an LED light source, two plate beamsplitters (PB2 and PB3), and a CCD camera for initial spot position determination. During the measurements, the plate beamsplitters were lifted up from the optical path to ensure optimal signal detection.

In the SMOKE measurements, it was customary to employ a slightly higher frequency than that used in electrical transport measurements [2–5]. This adjustment was made to improve the signal-to-noise ratio by minimizing the introduction of low-frequency vibration noise from the environment, such as that from the pulse tube refrigerator and the turbo molecular pump, into the SMOKE measurements. In this work, the AC current frequency employed in the SMOKE measurements was 1177 Hz, derived from the signal output of the lock-in amplifier. Figure S6 presents the MOKE and SMOKE measurements with current applied along the $b$-axis, while Figure S7 demonstrates the reproducibility of the nonlinear SMOKE signal across multiple $WTe_2$ devices.

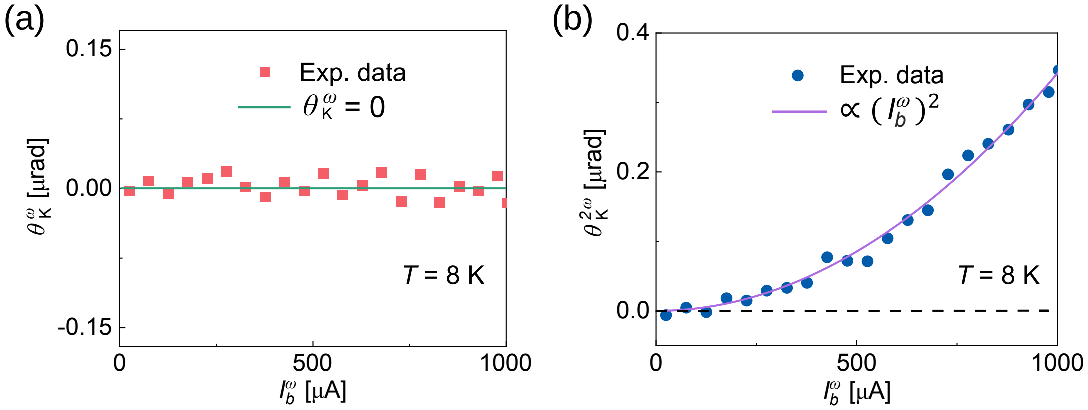


FIG. S6. MOKE and SMOKE with current along the $b$ axis. (a) The MOKE signal $\theta_K^\omega$ as a function of current $I^\omega$ applied along the $b$ axis. No signal was detected within the measurement accuracy. (b) The SMOKE signal $\theta_K^{2\omega}$ as a function of current $I_b^\omega$, fitted with a quadratic curve (purple solid line).

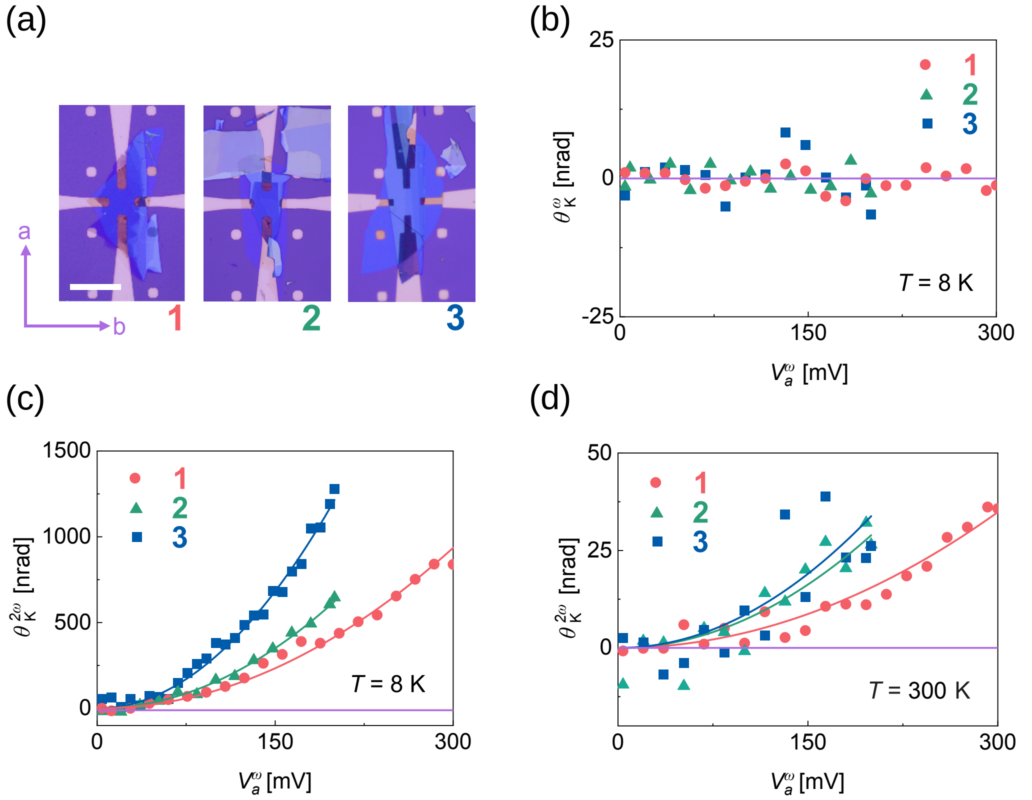


FIG. S7. Reproducibility of the nonlinear SMOKE signal across multiple $WTe_2$ devices. (a) Optical images of three representative $WTe_2$ devices from different batches. The scale bar is 30 $\mu$m. (b) MOKE signal $\theta_K^\omega$ as a function of $V_a^\omega$ for the three devices at 8 K, showing no detectable signal within the measurement resolution. (c) SMOKE signal $\theta_K^{2\omega}$ for the same devices at 8 K. The solid curves are quadratic fits to the data, confirming the nonlinear nature of the response. (d) SMOKE signal $\theta_K^{2\omega}$ measured at 300 K, demonstrating that a finite nonlinear response persists at room temperature in the devices. The solid curves are quadratic fits.

## SVI. EXPERIMENTAL DATA IN GRAPHENE CONTROL DEVICE

To rule out spurious nonlinear optical effects (such as the electro-optic Kerr effect) and current-induced heating artifacts as the origin of the observed SMOKE signal, we performed a control experiment using a graphene device [Fig. S8(a)]. This device, covered with an h-BN protective layer, was fabricated using an identical process to that of

the $WTe_2$ devices, featuring the same electrode geometry and a similar flake thickness. The linear I-V characteristic of the graphene device [Fig. S8(b)] confirms high-quality ohmic contacts and yields a resistance of 207 Ω, which is comparable to that of our $WTe_2$ devices, ensuring similar current density and similar levels of Joule heating during measurement.

Crucially, and in contrast to $WTe_2$, we observed neither a MOKE nor a SMOKE signal in the graphene device at room temperature, as shown in Figs. S8(c) and (d). This null result is decisive for two key reasons. First, graphene possesses a centrosymmetric crystal structure, which forbids the generation of a second-order nonlinear magnetization, consistent with our observations. Second, graphene is known to have one of the largest third-order nonlinear susceptibilities among all two-dimensional materials [6]. If the signal in $WTe_2$ were driven by a conventional optical nonlinearity like the electro-optic Kerr effect, a comparable or even stronger signal would be expected in graphene under the same excitation conditions. The complete absence of a signal in graphene therefore conclusively excludes both the electro-optic Kerr effect and current-induced heating as possible origins, firmly establishing the intrinsic and symmetry-enabled nature of the nonlinear magnetization observed in $WTe_2$. Figs. S8(e) and (f) depict the nonlinear voltages parallel ($V_{\parallel}^{2\omega}$) and perpendicular ($V_{\perp}^{2\omega}$) to the direction of $I_{\parallel}^{\omega}$, respectively. As $I_{\parallel}^{\omega}$ increases, both directions exhibit a clear quadratic current-voltage characteristic. Notably, $V_{\parallel}^{2\omega}$ is approximately five times larger than $V_{\perp}^{2\omega}$, which is distinctly different from the response observed in the nonlinear Hall effect induced by the Berry curvature dipole, where only a Hall response is present and the longitudinal response is absent. In the graphene/h-BN device, the nonlinearity likely stems from the interface contact between these two materials, as reported in reference [7].

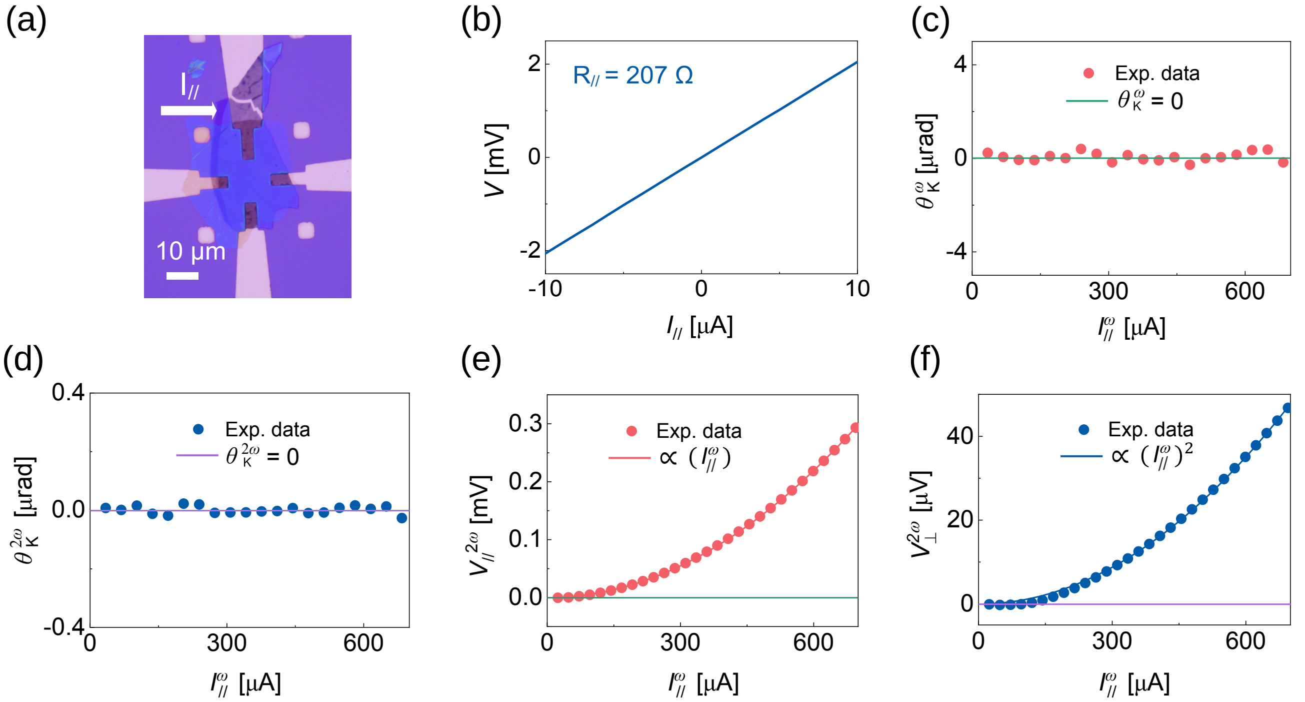


FIG. S8. Control measurements on a graphene device. (a) Optical image of the graphene control device. (b) I-V characteristic, showing linear ohmic behavior with a fitted resistance of 207 Ω. (c) Measurement of the MOKE signal $\theta_K^{\omega}$ shows no detectable response. (d) Measurement of the SMOKE signal $\theta_K^{2\omega}$ also shows no detectable response. (e) The nonlinear longitudinal voltage $V_{\parallel}^{2\omega}$ as functions of the current $I_{\parallel}^{\omega}$. (f) The nonlinear transverse voltage $V_{\perp}^{2\omega}$ as functions of the current $I_{\parallel}^{\omega}$. The solid lines in (e) and (f) represent quadratic fits to the experimental data.

## SVII. LASER INTENSITY DEPENDENCE OF THE SMOKE

To exclude laser-induced heating as a possible origin of the nonlinear SMOKE signal, we systematically investigated its dependence on incident laser power at 8 K. As shown in Fig. S9(a), the SMOKE signal maintains a clean quadratic dependence on the applied current across all tested laser power levels. To further quantify the laser power dependence, the signal amplitudes at two fixed current values, $I_{\mathrm{a}}^{\omega} = 260\,\mu$A and $910\,\mu$A, were directly extracted from the experimental data and plotted as a function of laser power in Fig. S9(b). The resulting amplitudes show no systematic variation with laser intensity, providing direct evidence that the nonlinear response is independent of optical power. This lack of correlation decisively rules out thermal effects driven by optical absorption, confirming that the laser acts solely as a passive probe.

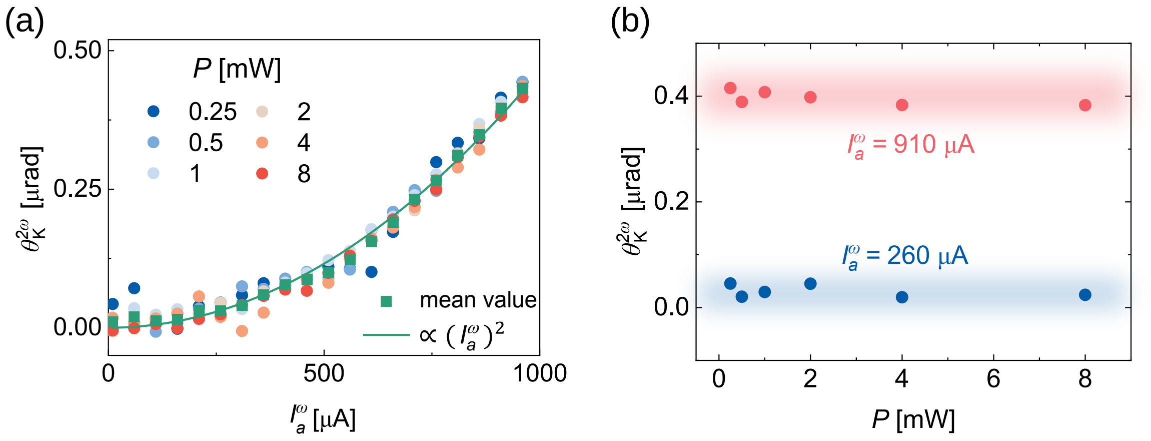


FIG. S9. Laser intensity dependence of the SMOKE. (a) The SMOKE signal $\theta_{\mathrm{K}}^{2\omega}$ as a quadratic function of applied current across varying laser intensities. (b) The SMOKE signal $\theta_{\mathrm{K}}^{2\omega}$ at different laser intensities with a fixed current of $I_{\mathrm{a}}^{\omega} = 260\,\mu$A and $910\,\mu$A, respectively.

## SVIII. THEORY OF NONLINEAR MAGNETIZATION

### A. Boltzmann Kinetics for Non-equilibrium Distribution Function

We adopt Boltzmann kinetics to obtain coefficient $\alpha_{ijk}$. For the electron evolution in the phase space, it is desirable to introduce the non-equilibrium distribution function $f(\mathbf{r}, \mathbf{k}, t)$, which satisfies [8–10]

$$\frac{\partial f}{\partial t} + \dot{\mathbf{r}} \cdot \nabla f + \dot{\mathbf{k}} \cdot \frac{\partial f}{\partial \mathbf{k}} = \mathcal{I}\{f\}. \tag{S3}$$

where $\mathcal{I}\{f\}$ is the deviation of distribution function due to collisions. At the steady state, $\partial_t f = 0$. For a uniform perturbation, we drop the spatial gradient term. Now, the distribution function $f$ satisfies

$$\dot{\mathbf{k}} \cdot \frac{\partial f}{\partial \mathbf{k}} = \mathcal{I}\{f\}. \tag{S4}$$

It is the celebrated Boltzmann equation for electrons under electric field. The left side is called drift term, while the right side is collision term. It is usually assumed that the non-equilibrium distribution deviates less from the equilibrium distribution. We shall assume a simple relaxation time approximation

$$\mathcal{I}\{f\} \simeq -\frac{f - f_0}{\tau}, \tag{S5}$$

where $\tau$ is the scattering time.

Now, under the electric field, i.e., $\dot{\mathbf{k}} = -e\mathbf{E}/\hbar$, the Boltzmann equation becomes

$$\begin{aligned} &\frac{-e}{\hbar}\mathbf{E} \cdot \partial_{\mathbf{k}} f = -\frac{f - f_0}{\tau}, \\ \Rightarrow\ &\left(1 - \frac{\tau e}{\hbar}\mathbf{E} \cdot \partial_{\mathbf{k}}\right) f = f_0, \\ \Rightarrow\ &(1 - \mathcal{Q}) f = f_0, \end{aligned} \tag{S6}$$

where the operator $\mathcal{Q}$ defined as $\mathcal{Q} \equiv (\tau e/\hbar)\mathbf{E}\cdot\partial_{\mathbf{k}}$. Accordingly, we can obtain the solution as

$$f = \frac{1}{1-\mathcal{Q}} f_0 = \sum_{\nu} \mathcal{Q}^{\nu} f_0. \tag{S7}$$

The zeroth-order term is just $f_0$, the first-order and second-order terms are evidently

$$\begin{cases} f_1 = \dfrac{\tau e}{\hbar}\mathbf{E}\cdot\partial_{\mathbf{k}} f_0, \\ f_2 = \left(\dfrac{\tau e}{\hbar}\mathbf{E}\cdot\partial_{\mathbf{k}}\right)^2 f_0, \end{cases} \tag{S8}$$

while the $\nu$-th order term is given by

$$f_{\nu} = \mathcal{Q}^{\nu} f_0 = \left(\frac{\tau e}{\hbar}\mathbf{E}\cdot\partial_{\mathbf{k}}\right)^{\nu} f_0. \tag{S9}$$

Explicitly, by using the non-equilibrium distribution function, we have the response of a measurable quantity $\mathcal{S}$ as

$$\mathcal{R} = \frac{1}{\mathcal{V}}\sum_{n,\mathbf{k}} \langle \mathcal{S}\rangle f = \int [d\mathbf{k}] \langle \mathcal{S}\rangle f, \tag{S10}$$

where we have replaced the sum over $\mathbf{k}$ by the integral, and $[d\mathbf{k}]$ represents $\sum_n d^d\mathbf{k}/(2\pi)^d$ with dimension $d$ and band index $n$.

### B. Calculation of Nonlinear Spin Magnetization Coefficient

The spin magnetization is given by the integral of the spin moment $\tilde{\mathbf{m}}_n^{\mathrm{S}}$ carried by the Bloch states weighted by the distribution function $f$, which is written as

$$\mathbf{M}^{\mathrm{S}} = \int [d\mathbf{k}] \tilde{\mathbf{m}}_n^{\mathrm{S}} f. \tag{S11}$$

The total spin moment has two origins, the first is the expectation value of the spin operator for the Bloch state $|n\rangle$ (shorthand of $|u_n(\mathbf{k})\rangle$), and the second is the anomalous correction linear to the electric field

$$\tilde{\mathbf{m}}_n^{\mathrm{S}} = \mathbf{m}_n^{\mathrm{S}} + \mathbf{m}_n^{\mathrm{S},(1)} = -g\mu_B \langle n| \mathbf{s} |n\rangle + e\mathbf{F}_n^{\mathrm{S}}\cdot\mathbf{E}, \tag{S12}$$

where $g$ is the Landé g factor for spin, $\mu_B = e\hbar/(2m)$ is the Bohr Magneton, $\mathbf{s} = \boldsymbol{\sigma}/2$ is the dimensionless spin operator, $-e$ is the electron charge, $m$ is the electron mass, and $\mathbf{F}_n^{\mathrm{S}}$ is the spin polarizability tensor given by [11]

$$F_n^{\mathrm{S},ij} = 2g\mu_B \mathrm{Im}\sum_{m\neq n} \frac{\langle n|s_i|m\rangle\langle m|\partial_j\mathcal{H}|n\rangle}{(\varepsilon_n - \varepsilon_m)^2}, \tag{S13}$$

where $\partial_i$ represents $\partial/(\partial k_i)$, which is a time-reversal odd tensor, i.e., $\mathcal{T}^{\dagger} F_n^{\mathrm{S},ij}(\mathbf{k})\mathcal{T} = -F_n^{\mathrm{S},ij}(-\mathbf{k})$.

Up to the second order of electric field, the distribution function is given by [Eq. (S8)]

$$f = f_0 + \frac{\tau e}{\hbar}\mathbf{E}\cdot\partial_{\mathbf{k}} f_0 + \left(\frac{\tau e}{\hbar}\mathbf{E}\cdot\partial_{\mathbf{k}}\right)^2 f_0. \tag{S14}$$

Considering the correction of energy [12–14], the Fermi distribution function $f_0$ is now a function of electric field $\mathbf{E}$. To obtain the nonlinear response, we expand $f_0$ as a series

$$f_0(\varepsilon_n + \frac{e}{2}\mathbf{E}\cdot\mathbf{G}_n\cdot\mathbf{E}) \simeq f_0(\varepsilon_n) + \frac{e}{2}\mathbf{E}\cdot\mathbf{G}_n\cdot\mathbf{E} f_0', \tag{S15}$$

where $\mathbf{G}_n$ is the the Berry connection polarizability tensor given by

$$G_n^{ij} = 2e\mathrm{Re}\sum_{m\neq n} \frac{\langle n|\partial_i\mathcal{H}|m\rangle\langle m|\partial_j\mathcal{H}|n\rangle}{(\varepsilon_n - \varepsilon_m)^3}, \tag{S16}$$

which is a time-reversal even tensor, i.e., $\mathcal{T}^\dagger G_n^{ij}(\mathbf{k})\mathcal{T} = F_n^{\mathrm{S},ij}(-\mathbf{k})$.

By substituting the expression of $f$ [Eq. (S14)] into Eq. (S11), and retaining terms up to the square of the electric field, we can obtain that

$$\begin{aligned} M_i^{\mathrm{S}} &= \int [d\mathbf{k}] \tilde{m}_n^{\mathrm{S},i} f \\ &= \int [d\mathbf{k}](-g\mu_B s_n^i + eF_n^{\mathrm{S},ij}E_j)\Big[f_0 + \frac{e}{2}G_n^{jk}E_jE_kf_0' + \frac{\tau e}{\hbar}E_j\partial_j f_0 + \Big(\frac{\tau^2 e^2}{\hbar^2}E_jE_k\partial_j\partial_k\Big)f_0\Big] \\ &= \int [d\mathbf{k}]\Big[-g\mu_B s_n^i\big(f_0 + \frac{e}{2}G_n^{jk}f_0'E_jE_k + \frac{\tau e}{\hbar}\partial_j f_0 E_j + \frac{\tau^2 e^2}{\hbar^2}\partial_j\partial_k f_0 E_jE_k\big) + eF_n^{\mathrm{S},ij}f_0E_j \\ &\quad + eF_n^{\mathrm{S},ij}\frac{\tau e}{\hbar}\partial_k f_0 E_jE_k\Big], \end{aligned} \tag{S17}$$

where we have denoted $s_n^i = \langle n|\, s_i\, |n\rangle$. According to the order of electric field $\mathbf{E}$, the spin magnetization $\mathbf{M}^{\mathrm{S}}$ can be divided into three contributions, the first is the spin magnetization of ground state

$$M_i^{\mathrm{S},(0)} = -g\mu_B \int [d\mathbf{k}] s_n^i f_0, \tag{S18}$$

which vanishes with time-reversal symmetry. The second contribution is linear to the electric field, given by

$$\begin{aligned} M_i^{\mathrm{S},(1)} &= \int [d\mathbf{k}]\Big[(-g\mu_B s_n^i)\frac{\tau e}{\hbar}\partial_j f_0 + eF_n^{\mathrm{S},ij}f_0\Big]E_j \\ &= \int [d\mathbf{k}]\big[(-g\mu_B s_n^i)\tau e v_n^j f_0' + eF_n^{\mathrm{S},ij}f_0\big]E_j, \end{aligned} \tag{S19}$$

where $\mathbf{v}_n = \partial_{\mathbf{k}}\varepsilon_n/\hbar$, and only the first term retains with time-reversal symmetry. The third contribution is a nonlinear response which is in second order of electric fields, given by

$$\begin{aligned} M_i^{\mathrm{S},(2)} &= \int [d\mathbf{k}]\Big[(-g\mu_B s_n^i)\Big(\frac{e}{2}G_n^{jk}f_0' + \frac{\tau^2 e^2}{\hbar^2}\partial_j\partial_k f_0\Big) + eF_n^{\mathrm{S},ij}\frac{\tau e}{\hbar}\partial_k f_0\Big]E_jE_k \\ &= \int [d\mathbf{k}]\Big[(-g\mu_B s_n^i)\Big(\frac{e}{2}G_n^{jk}f_0' + \frac{\tau^2 e^2}{\hbar}\partial_j v_n^k f_0'\Big) + \tau e^2 F_n^{\mathrm{S},ij}v_n^k f_0'\Big]E_jE_k, \end{aligned} \tag{S20}$$

where, under time-reversal symmetry, only the last term remains.

In summary, for the system with time-reversal symmetry, i.e., non-magnetic system, the nonlinear spin magnetization coefficient is given by

$$\alpha_{ijk}^{\mathrm{S}} = \tau e^2 \int [d\mathbf{k}] F_n^{\mathrm{S},ij} v_n^k f_0'. \tag{S21}$$

### C. Calculation of Nonlinear Orbital Magnetization Coefficient

Similar to the spin case, the orbital magnetization is given by

$$\mathbf{M}^{\mathrm{O}} = \int [d\mathbf{k}] \tilde{\mathbf{m}}_n^{\mathrm{O}} f. \tag{S22}$$

The total orbital moment also has two origins, the first is the intrinsic orbital moment of the Bloch state, and the second is the anomalous correction linear in the electric field

$$\tilde{\mathbf{m}}_n^{\mathrm{O}} = \mathbf{m}_n^{\mathrm{O}} + \mathbf{m}_n^{\mathrm{O},(1)} = \mathbf{m}_n^{\mathrm{O}} + e\mathbf{F}_n^{\mathrm{O}}\cdot\mathbf{E}. \tag{S23}$$

Here, $\mathbf{m}_n^{\mathrm{O}}$ is the intraband orbital moment given by

$$m_n^{\mathrm{O},i} = -\epsilon_{ijk}\frac{e}{\hbar}\mathrm{Im}\sum_{m\neq n}\frac{\langle n|\partial_j\mathcal{H}|m\rangle\langle m|\partial_k\mathcal{H}|n\rangle}{\varepsilon_n - \varepsilon_m} \tag{S24}$$

with full anti-symmetric tensor $\epsilon_{ijk}$, which is time-reversal odd, i.e., $\mathcal{T}^\dagger m_n^{\mathrm{O},i}(\mathbf{k})\mathcal{T} = -m_n^{\mathrm{O},i}(-\mathbf{k})$; $\mathbf{F}_n^{\mathrm{O}}$ is the orbital polarizability tensor given by [12]

$$F_n^{\mathrm{O},ij} = -2\mathrm{Im}\sum_{m\neq n}\frac{m_{nm}^{\mathrm{O},i}\langle m|\partial_j\mathcal{H}|n\rangle}{(\varepsilon_n-\varepsilon_m)^2} - \frac{e}{2\hbar}\epsilon_{ikl}\partial_k g_n^{lj}. \tag{S25}$$

which is time-reversal odd, i.e., $\mathcal{T}^\dagger F_n^{\mathrm{O},ij}(\mathbf{k})\mathcal{T} = -F_n^{\mathrm{O},ij}(-\mathbf{k})$, where $\mathbf{m}_{mn}^{\mathrm{O}}$ is the inter-band element of the orbital moment

$$m_{mn}^{\mathrm{O},i} = \frac{ie}{2\hbar}\epsilon_{ijk}\Big[\sum_{p\neq n}\frac{\langle m|\partial_j\mathcal{H}|p\rangle\langle p|\partial_k\mathcal{H}|n\rangle}{\varepsilon_n-\varepsilon_p} + \frac{\langle n|\partial_j\mathcal{H}|n\rangle\langle m|\partial_k\mathcal{H}|n\rangle}{\varepsilon_n-\varepsilon_m}\Big], \tag{S26}$$

and $g_n^{ij}$ is the quantum metric tensor given by

$$g_n^{ij} = \mathrm{Re}\sum_{m\neq n}\frac{\langle n|\partial_i\mathcal{H}|m\rangle\langle m|\partial_j\mathcal{H}|n\rangle}{(\varepsilon_n-\varepsilon_m)^2}, \tag{S27}$$

which is time-reversal even, i.e., $\mathcal{T}^\dagger g_n^{ij}(\mathbf{k})\mathcal{T} = g_n^{ij}(-\mathbf{k})$. We remark that $\epsilon_{ikl}\partial_k g_n^{lj}$ in $F_n^{\mathrm{O},ij}$ can be written as

$$\epsilon_{ikl}\partial_k g_n^{lj} = \frac{1}{2}\epsilon_{ikl}(\partial_k g_n^{lj} - \partial_l g_n^{kj}) = \frac{1}{2}\epsilon_{ikl}(\partial_j g_n^{kl} + \partial_k g_n^{lj} - \partial_l g_n^{kj}) = \epsilon_{ikl}\Gamma_n^{lkj}, \tag{S28}$$

where we have used $\epsilon_{ikl}\partial_j g_n^{kl} = 0$ and $\Gamma_n^{lkj} = (\partial_j g_n^{kl} + \partial_k g_n^{lj} - \partial_l g_n^{kj})/2$ is the Christoffel symbol. Thus, $\mathbf{F}_n^{\mathrm{O}}$ becomes

$$F_n^{\mathrm{O},ij} = -2\mathrm{Im}\sum_{m\neq n}\frac{m_{nm}^{\mathrm{O},i}\langle m|\partial_j\mathcal{H}|n\rangle}{(\varepsilon_n-\varepsilon_m)^2} - \frac{e}{2\hbar}\epsilon_{ikl}\Gamma_n^{lkj}. \tag{S29}$$

By substituting the expression of $f$ [Eq. (S14)] into Eq. (S22) and retaining terms up to the square of the electric field, we can obtain that

$$\begin{aligned}
M_i^{\mathrm{O}} &= \int[d\mathbf{k}]\tilde{m}_n^{\mathrm{O},i}f \\
&= \int[d\mathbf{k}](m_n^{\mathrm{O},i} + eF_n^{\mathrm{O},ij}E_j)\Big[f_0 + \frac{e}{2}G_n^{jk}E_jE_kf_0' + \frac{\tau e}{\hbar}E_j\partial_jf_0 + \Big(\frac{\tau^2e^2}{\hbar^2}E_jE_k\partial_j\partial_k\Big)f_0\Big] \\
&= \int[d\mathbf{k}]\Big[m_n^{\mathrm{O},i}\big(f_0 + \frac{e}{2}G_n^{jk}f_0'E_jE_k + \frac{\tau e}{\hbar}\partial_jf_0E_j + \frac{\tau^2e^2}{\hbar^2}\partial_j\partial_kf_0E_jE_k\big) + eF_n^{\mathrm{O},ij}f_0E_j \\
&\quad + eF_n^{\mathrm{O},ij}\frac{\tau e}{\hbar}\partial_kf_0E_jE_k\Big].
\end{aligned} \tag{S30}$$

According to the order of electric field $\mathbf{E}$, the orbital magnetization $\mathbf{M}^{\mathrm{O}}$ can be divided into three contributions, the first is the orbital magnetization of ground state

$$M_i^{\mathrm{O},(0)} = \int[d\mathbf{k}]m_n^{\mathrm{O},i}f_0, \tag{S31}$$

which vanishes with time-reversal symmetry. The second contribution is linear to the electric field, written as

$$\begin{aligned}
M_i^{\mathrm{O},(1)} &= \int[d\mathbf{k}]\Big(m_n^{\mathrm{O},i}\frac{\tau e}{\hbar}\partial_jf_0 + eF_n^{\mathrm{O},ij}f_0\Big)E_j \\
&= \int[d\mathbf{k}]\big(m_n^{\mathrm{O},i}\tau ev_n^jf_0' + eF_n^{\mathrm{O},ij}f_0\big)E_j,
\end{aligned} \tag{S32}$$

where $\mathbf{v}_n = \partial_{\mathbf{k}}\varepsilon_n/\hbar$, and only the first term retains with time-reversal symmetry. The third contribution is a nonlinear response which is in second order of electric field, given by

$$\begin{aligned}
M_i^{\mathrm{O},(2)} &= \int[d\mathbf{k}]\Big[m_n^{\mathrm{O},i}\Big(\frac{e}{2}G_n^{jk}f_0' + \frac{\tau^2e^2}{\hbar^2}\partial_j\partial_kf_0\Big) + eF_n^{\mathrm{O},ij}\frac{\tau e}{\hbar}\partial_kf_0\Big]E_jE_k \\
&= \int[d\mathbf{k}]\Big[m_n^{\mathrm{O},i}\Big(\frac{e}{2}G_n^{jk}f_0' + \frac{\tau^2e^2}{\hbar}\partial_jv_n^kf_0'\Big) + \tau e^2F_n^{\mathrm{O},ij}v_n^kf_0'\Big]E_jE_k,
\end{aligned} \tag{S33}$$

where, under time-reversal symmetry, only the last term remains.

In summary, for the system with time-reversal symmetry, i.e., non-magnetic system, the nonlinear orbital magnetization coefficient is given by

$$\alpha_{ijk}^{\mathrm{O}} = \tau e^2\int[d\mathbf{k}]F_n^{\mathrm{O},ij}v_n^kf_0'. \tag{S34}$$

## SIX. ESTIMATION OF SCATTERING TIME

To determine the value of nonlinear magnetization coefficient $\alpha_{ijk}$ in Eq. (1) of the main text, we additionally need the scattering time $\tau$, which can be estimated by using the linear Drude conductivity

$$\sigma_{ij} = -e^2\tau \int [d\mathbf{k}] v_n^i v_n^j f_0'. \tag{S35}$$

For our effective model [Eq. (2) in the main text], we numerically calculate the Drude conductivity $\sigma_{xx}$ at 8 K. The result is shown in Fig. S10. In the experiment Fig. S3, the resistivity along the $a$ axis at 8 K is 80.77 Ω. This resistivity corresponds to $\tau \simeq 1.4$, 1.1, and 0.8 ps at $\varepsilon_F = 0.2$ eV for $t/v$ =0, 0.3, and 0.5, respectively.

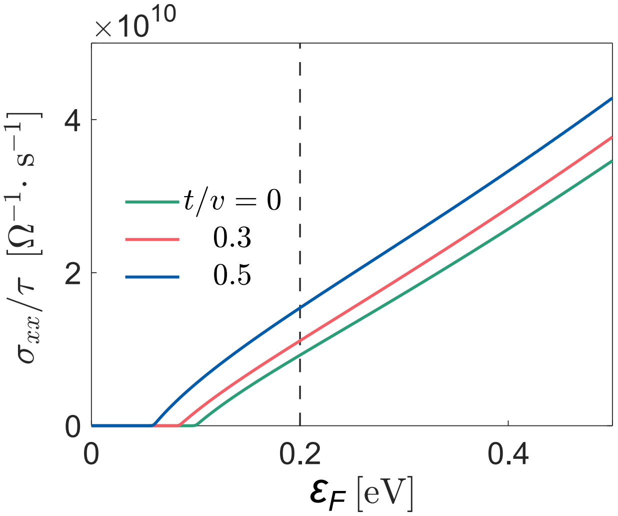


FIG. S10. Fermi energy dependence of the Drude conductivity. Different colors represent different values of $t$, while the other parameters are the same as those in Fig. 4 of the main text.


[1] I. H. Kao, R. Muzzio, H. Zhang, M. Zhu, J. Gobbo, S. Yuan, D. Weber, R. Rao, J. Li, J. H. Edgar, *et al.*, Deterministic switching of a perpendicularly polarized magnet using unconventional spin-orbit torques in $WTe_2$, Nat. Mater. **21**, 1029 (2022).

[2] C. Stamm, C. Murer, M. Berritta, J. Feng, M. Gabureac, P. M. Oppeneer, and P. Gambardella, Magneto-Optical Detection of the Spin Hall Effect in Pt and W Thin Films, Phys. Rev. Lett. **119**, 087203 (2017).

[3] Y.-G. Choi, D. Jo, K.-H. Ko, D. Go, K.-H. Kim, H. G. Park, C. Kim, B.-C. Min, G.-M. Choi, and H.-W. Lee, Observation of the orbital Hall effect in a light metal Ti, Nature **619**, 52 (2023).

[4] I. Lyalin, S. Alikhah, M. Berritta, P. M. Oppeneer, and R. K. Kawakami, Magneto-Optical Detection of the Orbital Hall Effect in Chromium, Phys. Rev. Lett. **131**, 156702 (2023).

[5] I. Lyalin and R. K. Kawakami, Interface transparency to orbital current, Phys. Rev. B **110**, 104418 (2024).

[6] Z. Xie, T. Zhao, X. Yu, and J. Wang, Nonlinear Optical Properties of 2D Materials and their Applications, Small **20**, 2311621 (2024).

[7] P. He, G. Koon, H. Isobe, J. Tan, J. Hu, A. Neto, L. Fu, and H. Yang, Graphene moiré superlattices with giant quantum nonlinearity of chiral Bloch electrons, Nat. Nanotechnol. **17**, 378 (2022).

[8] Hurd, *The Hall effect in metals and alloys* (Plenum Press, 1972).

[9] Ashcroft and Mermin, *Solid state physics* (Thomson Learning, 1976).

[10] H. Haug and A.-P. Jauho, *Quantum kinetics in transport and optics of semiconductors* (Springer, 2008).

[11] C. Xiao, W. Wu, H. Wang, Y.-X. Huang, X. Feng, H. Liu, G.-Y. Guo, Q. Niu, and S. A. Yang, Time-Reversal-Even Nonlinear Current Induced Spin Polarization, Phys. Rev. Lett. **130**, 166302 (2023).

[12] Y. Gao, S. A. Yang, and Q. Niu, Field Induced Positional Shift of Bloch Electrons and Its Dynamical Implications, Phys. Rev. Lett. **112**, 166601 (2014).

[13] C. Wang, Y. Gao, and D. Xiao, Intrinsic Nonlinear Hall Effect in Antiferromagnetic Tetragonal CuMnAs, Phys. Rev. Lett. **127**, 277201 (2021).

[14] H. Liu, J. Zhao, Y.-X. Huang, W. Wu, X.-L. Sheng, C. Xiao, and S. A. Yang, Intrinsic Second-Order Anomalous Hall Effect and Its Application in Compensated Antiferromagnets, Phys. Rev. Lett. **127**, 277202 (2021).
